# Supplementary material for: Manifold Regularized Dynamic Network Pruning
Source: arXiv:2103.05861 source file (2021-03-10)
Supplement: Supplementary file 1 [file supp_sim.pdf]

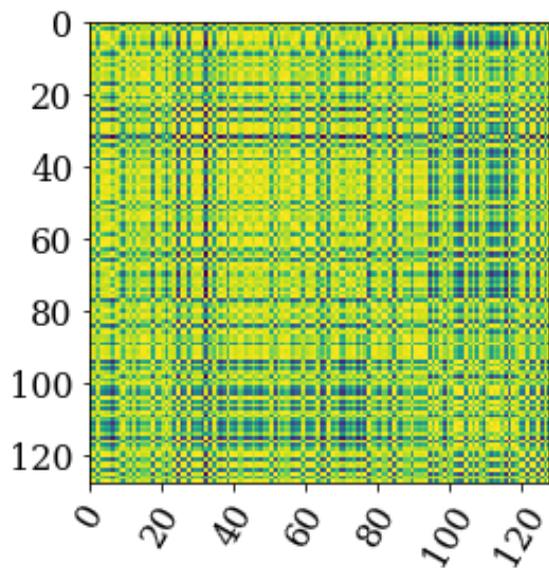

(a)

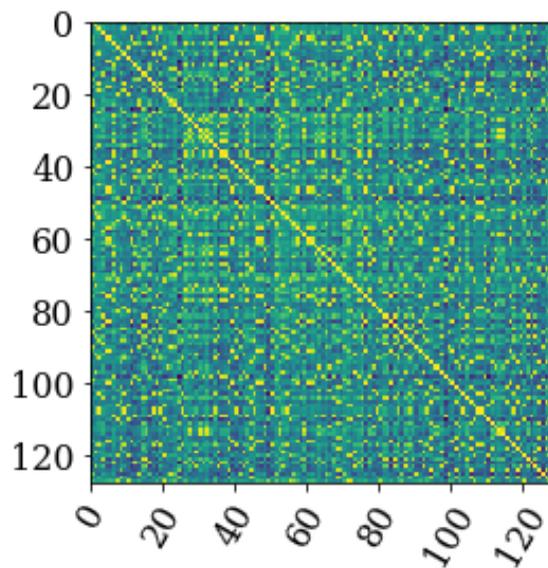

(b)

Without similarity loss

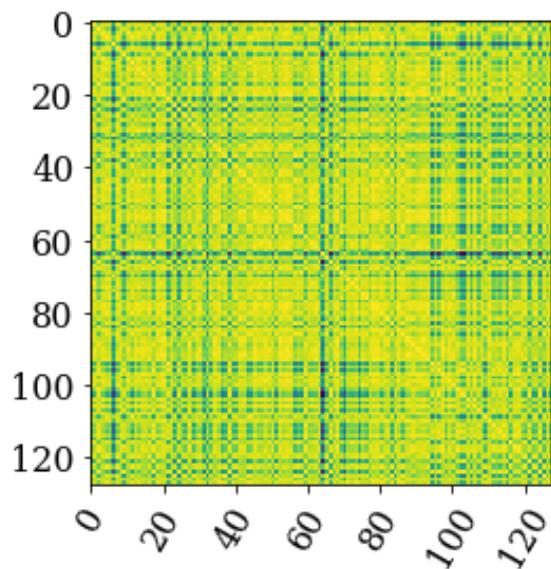

(c)

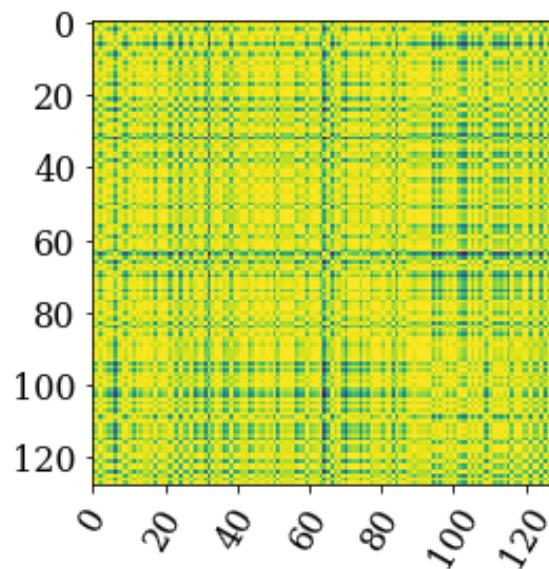

(d)

With similarity loss

Feature Similarity  
matrix with  $L_{sim}$

Mask

Mas  
k
