# Supplementary material for: Manifold Regularized Dynamic Network Pruning
Source: arXiv:2103.05861 source file (2021-03-10)

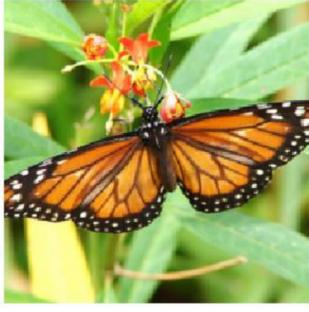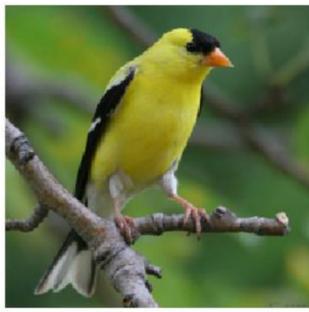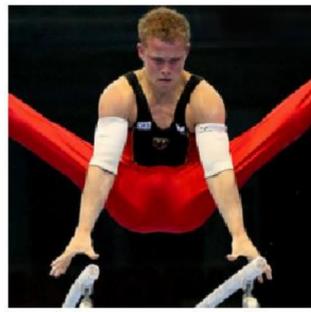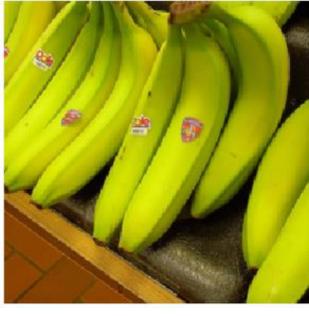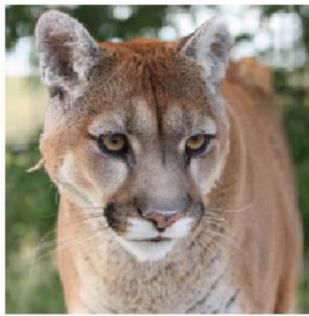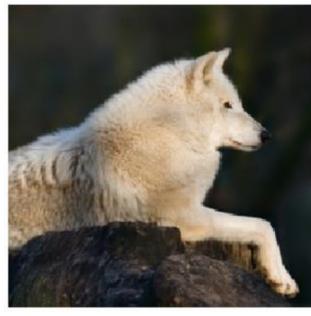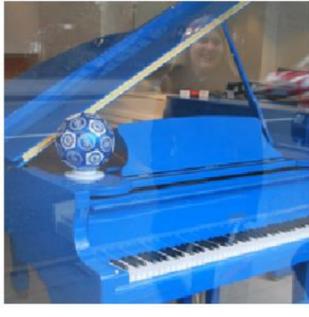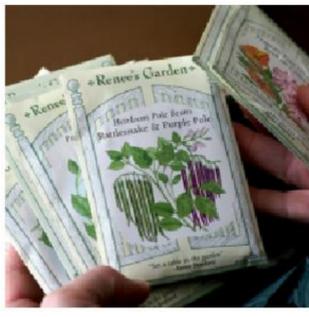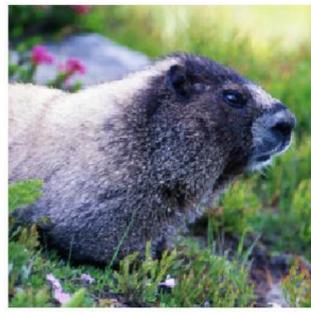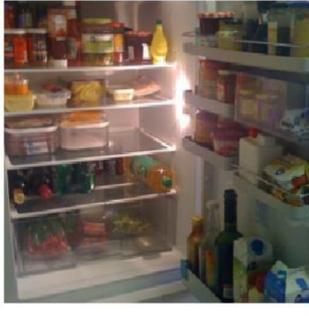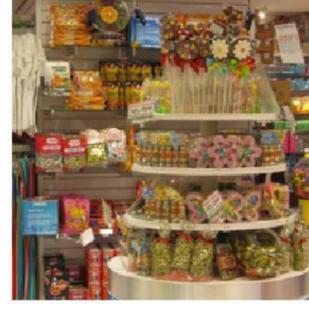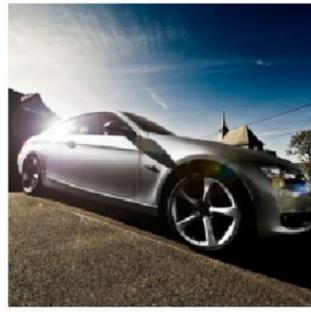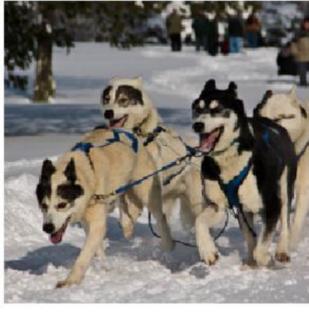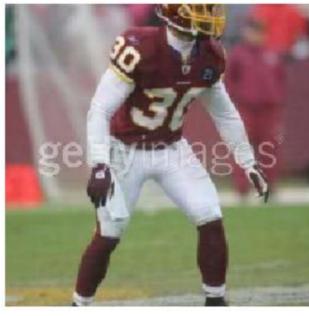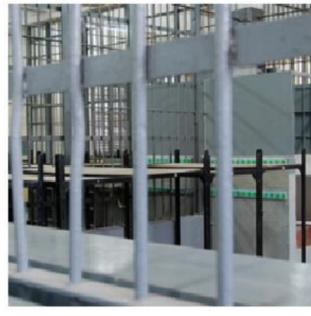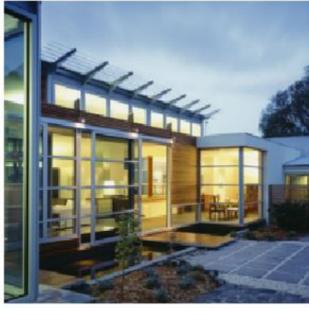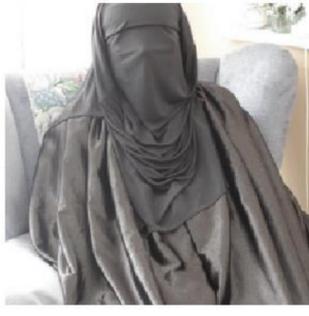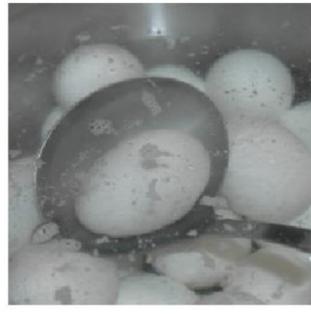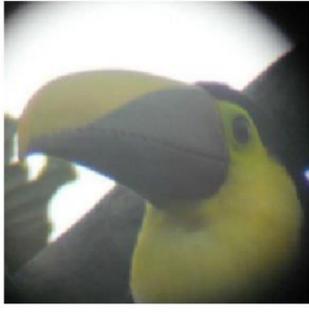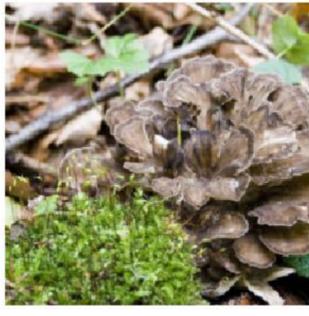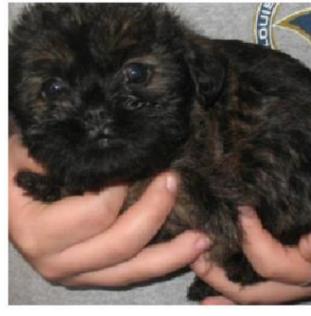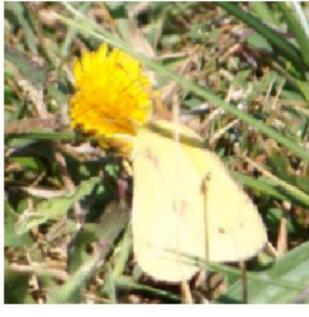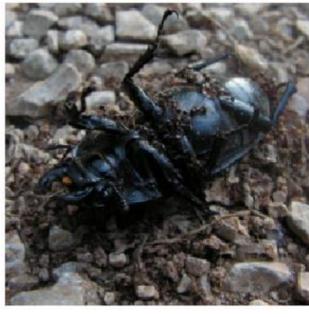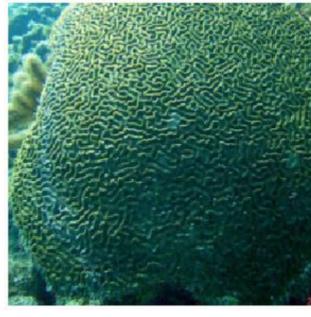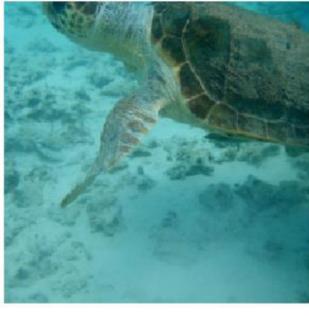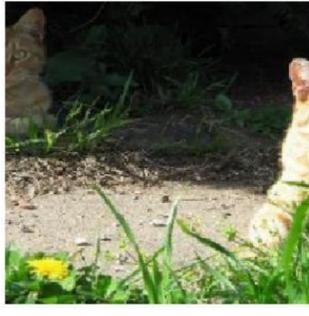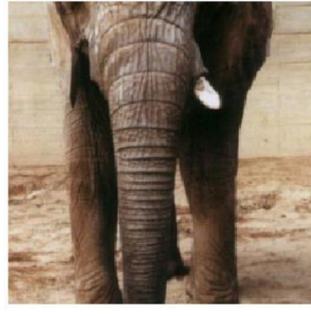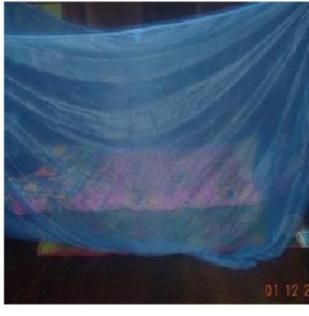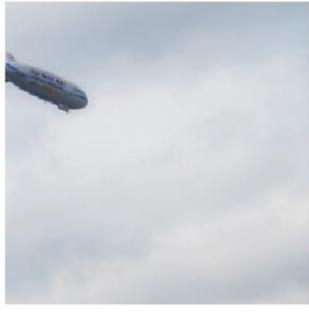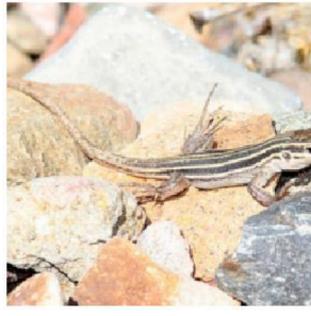

Complexity

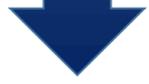

Supplement: Supplementary file 2 [file supp_visual.pdf]
